# Supplementary material for: Adversarial Resilience against Clean-Label Attacks in Realizable and Noisy Settings
Source: arXiv:2504.13966 source file (2025-04-17)
Supplement: Supplementary file 1 [file 08_Appendix.tex]

\begin{algorithm}[H]
    \caption{Learning in the Agnostic Setting with known distribution over $\mathcal{X}$}\label{alg:agnostic_shatter}
    \begin{algorithmic}[1]
        \State Set $S_0=\emptyset, i=0, \mathcal{F}_0=\mathcal{F}, k=d$
        \For{$t=1, \dots, T$}
        \State Receive $\hat{x}_t\in \mathcal{X}$
        \If{$k>0$}
        \State \textit{Learning based on $k$ shatterability like Algorithm \ref{alg:gen_vc}}
        \If{$\min\{\rho_k(\mathcal{F}_{i-1}^{\hat{x}_t\rightarrow 0}),\rho_k(\mathcal{F}_{i-1}^{\hat{x}_t\rightarrow 1})\}\geq 0.6\rho_k(\mathcal{F}_{i-1})$}
        \State $\hat{y}_t=\perp$
        \Else 
        \State predict $\hat{y}_t=\arg\max_{j\in\{0,1\}}\rho_k(\mathcal{F}_{i-1}^{\hat{x}_t\rightarrow j})$
        \State $\mathcal{F}_{i-1}\gets\mathcal{F}_{i-1}^{\hat{x}\rightarrow\hat{y}_t}$ \textit{Do we want to update here with the inferred label?}
        \EndIf        
        \State Receive the true label $y_t$ (where $y_t\sim P(\cdot |\hat{x}_t)$)
        \State update $S_i\gets S_i\cup \{(\hat{x}_t,y_t)\}$
        \If{$t=2^{i+1}$}
        \State  $\mathcal{F}_{i}\gets\{h\in \mathcal{F}_{i-1}: \text{er}_{S_i}(h)- \min_{f\in \mathcal{F}_{i-1}}\text{er}_{S_i}(f)\leq \alpha\}$
        \State update $i\gets i+1$, $S_i \gets \emptyset$
        \If{$\rho_k(\mathcal{F}_{i})\leq\alpha_k$}
        \State Set $k=k-1$
        \EndIf
        \EndIf
        \Else
        \State \textit{Disagreement based learning like in Algorithm \ref{alg:agnostic_disagree}}
        \If{$\hat{x}_t\in \mathcal{S}_1(\mathcal{F}_{i-1})$}
        \State $\hat{y}_t=\perp$
        \Else 
        \State predict $\hat{y}_t=f(\hat{x}_t)$ according to some $f\in\mathcal{F}_{i-1}$
        \EndIf
        \State Receive the true label $y_t$ (where $y_t\sim P(\cdot |\hat{x}_t)$)
        \State update $S_i\gets S_i\cup \{(\hat{x}_t,y_t)\}$
        \If{$t=2^{i+1}$}
        \State  $\mathcal{F}_{i}\gets\{h\in \mathcal{F}_{i-1}: \text{er}_{S_i}(h)- \min_{f\in \mathcal{F}_{i-1}}\text{er}_{S_i}(f)\leq \alpha\}$
        \State update $i\gets i+1$, $S_i \gets \emptyset$
        \EndIf
        \EndIf
        \EndFor
    \end{algorithmic}
\end{algorithm}
